# Supplementary material for: SplitBFT: Improving Byzantine Fault Tolerance Safety Using Trusted Compartments
Source: arXiv:2205.08938 source file (2022-05-24)
Supplement: Supplementary file 1 [file 08-appendix.tex]

\newpage

%% definitions
\newcommand{\prepareDigest}{$\langle$\prepare,\textit{v,n,$D(m)$,i}$\rangle \subrangle{\preparation}$ }
\newcommand{\prepreparej}{$\langle$\preprepare,\textit{v,n,m}$\rangle \subrangle{\preparation}$ }
\newcommand{\preparei}{$\langle$\prepare,\textit{v,n,d,i}$\rangle \subrangle{\preparation}$ }
\newcommand{\preparej}{$\langle$\prepare,\textit{v,n,d,j}$\rangle \subrangle{\preparation}$ }
\newcommand{\commiti}{$\langle$\commit,\textit{v,n,$D(m)$,i}$\rangle \subrangle{\confirmation}$ }

%\newcommand{\preparej}{$\langle$\prepare,\textit{v,n,d,j}$\rangle \subrangle{Epi}$ }

%\DrawBox[draw=orange,fill=orange!30]{c}{d}
\section{Appendix}

In this appendix, we present the original PBFT pseudocode~\cite{castrothesis} including annotations in which of our the three compartments the code is placed. \im{coloring}

%%%%%%%%%%%%%%%%%%%%%%%%%%%%%%%%%%
\newcommand\sendprepre[3][]{%
  \begin{tikzpicture}[remember picture,overlay]
    \draw[overlay,fill=green!30,#1] 
    ([xshift=2em,yshift=-9ex]{pic cs:#2}) 
    rectangle 
    ([xshift=6cm,yshift=9ex]pic cs:#3);
  \end{tikzpicture}%
}

%%%%%%%%%%%%%%%%%%%%%%%%%
 \scalebox{0.8}{
    \begin{minipage}{\linewidth}
\begin{algorithm}[H]
   % \caption{Text Summarization Algorithm}\label{euclid}
    \begin{algorithmic}[1]

\Procedure{\rec(\clientreq)}{} 
  \State Eff: let $m\gets $\clientreq$ $

\If{$t$= $last\mbox{-}rep\mbox{-}t_{i}(c)$ }
\State \mbox{$out_{i}:=out_{i}$ $\cup$ \{\replysig\} }
\ElsIf  {$t$ $>$ $last\mbox{-}rep\mbox{-}t_{i}(c)$ }
\State $in_{\preparation}:=in_{\preparation}$ $\cup$ \{$m$\}
 \If{ $primary(i)$ $\neq$ $I$}
\State $out_{\preparation}$:= $out_{\preparation}$ $\cup$ \{m\}
\EndIf
\EndIf
\EndProcedure

\end{algorithmic}
\end{algorithm}
\end{minipage}
}

%%%%%%%%%%%%%%%%%%%%%%%%%%%%%%%%%%%%%%%
 \scalebox{0.8}{
    \begin{minipage}{\linewidth}
\sendprepre{aa}{bb}
\begin{algorithm}[H]
   % \caption{Text Summarization Algorithm}\label{euclid}
    \begin{algorithmic}[1]

\Procedure{\textsc{send-pre-prepare}$(\textit{m,v,n})_{\preparation}$}{} 
% TODO: fix function
\State \mbox{Pre: enter\mbox{-}enclave($e_{\preparation}$) $\land$ load($in_{\preparation}$)$\land$ \prepenclave{ \textit{verif}(D( $in_{\preparation}$), $hash_{\preparation}$)}}

%\State \If{$verify_{Epi}$ (D( $in_{Epi}$),D(\hasnewview ))}

\State \mbox{$primary(\prepenclave{view_{\preparation}})$) = $i$ $\land$ \prepenclave{$se
qno_{\preparation}$}= n-1 $\land$  $\land$ \inwv $\land$ \hasnewview $\land$  }

\Indent\State \mbox{$\exists$ $o,t,c$: (m= \clientreq $\land$ m $\in$ $in_{\preparation}$) $\land$ $\nexists$ $\langle$\preprepare,\textit{v,n$'$,m}$\rangle \subrangle{\preparation}$ $\in$ $in_{\preparation}$}
\EndIndent
\State Eff:  $seqno_{\preparation}$=$seqno_{\preparation}$+1
\Indent

\State let p=
 $\langle$\preprepare,\textit{v,n,m}$\rangle \subrangle{\preparation}$

\State $in_{\preparation}:=in_{\preparation}$ $\cup$ \{$p$\}
%\State $load($in_{\preparation}$)$ $\land$update\mbox{-}hash(in_{\preparation})$
\State $hash:= update\mbox{-}hash(in_{\preparation})$
\State $exit\mbox{-}enclave($$e_{\preparation}$$)$
\State $out_{i}:=out_{i}$ $\cup$ \{$p$\}

%\State $updatehash(in_{Epi})$
\EndIndent
%\EndIf
\EndProcedure

\end{algorithmic}
\end{algorithm}
\end{minipage}}

%%%%%%%%%%%%%%%%%%%%%%%%%%%%%%%%%

%%%%%%%%%%%%%%%%%%%%%%%%%%%%%%%%%%
\newcommand\receiveprepre[3][]{%
  \begin{tikzpicture}[remember picture,overlay]
    \draw[overlay,fill=green!30,#1] 
    ([xshift=-26em,yshift=-1ex]{pic cs:#2}) 
    rectangle 
    ([xshift=11cm,yshift=-8ex]pic cs:#3);
  \end{tikzpicture}%
}

%%%%%%%%%%%%%%%%%%%%%%%%%%%%%%%%%%%%%%%
%%%%%%%%%%%%%%%%%%%%%%%%%%%%%%%%%%%%%%%%%%%%%%%%%%%%%%%%%%%%%%%%%

%\begin{frame}{Receive Pre-prepare}
 \scalebox{0.8}{
    \begin{minipage}{\linewidth}
\receiveprepre{cc}{dd}
\begin{algorithm}[H]
   % \caption{Text Summarization Algorithm}\label{euclid}
    \begin{algorithmic}[1]

\Procedure{\rec(\prepreparej)$_{i}$ ($i$ $\neq$ $j$)}{}
\tikzmark{bb}
\State \mbox{Eff: \nolinebreak }\If  {\mbox{j= $primary(view_{\preparation})$ $\land$ \inwv $\land$ \hasnewview } $\land$ \\ \hskip2.8em$\nexists$ $d$:  (d $\neq$ $D(m)$ $\land$ \preparei $\in$ $in_{\preparation}$) }
\EndIf 

\Indent
\State  let $p$= \prepareDigest
%// \prep{\textbf{signed by the preparation enclave in backup replicas}}
\State \hskip1em $in_{\preparation}:=in_{\preparation}$ $\cup$ \{\prepreparej, $p$\}
%\State \hskip1em $in_{\confirmation}:=in_{\confirmation}$ $\cup$ \{\prepreparej, $p$\}
\tikzmark{cc}
\State \hskip1em $out_{i}:=out_{i}$ $\cup$ \{$p$\}

\EndIndent 

\EndProcedure

\end{algorithmic}
\end{algorithm}
\end{minipage}
}
%\end{frame}

%%%%%%%%%%%%%%%%%%%%%%%%%%%%%%%%%%%%%

%%%%%%%%%%%%%%%%%%%%%%%%%%%%%%%%%%%%%%%%%

\newcommand\receiveprepare[3][]{%
  \begin{tikzpicture}[remember picture,overlay]
    \draw[overlay,fill=blue!30,#1] 
    ([xshift=-23em,yshift=-1.5ex]{pic cs:#2}) 
    rectangle 
    ([xshift=9cm,yshift=0.1ex]pic cs:#3);
  \end{tikzpicture}%
}

%%%%%%%%%%%%%%%%%%%%%%%%%%%%%%%%%%%%%%%%%
%\begin{frame}{Receive Prepare}

% \begin{itemize}
% \item $in\hbox{-}v (v,i)$ $\equiv$ $view_{i}$= v 
% \end{itemize}
 \receiveprepare{ee}{ff}
\scalebox{0.8}{
    \begin{minipage}{\linewidth}
\begin{algorithm}[H]
   % \caption{Text Summarization Algorithm}\label{euclid}
    \begin{algorithmic}[1]

\Procedure{\rec(\preparej)$_{i}$ ($i$ $\neq$ $j$)}{}
\tikzmark{ee}
\State  Eff: \If  {j$\neq$ $primary($$view_{\confirmation}$$)$ $\land$ v $\geq$ $view_{\confirmation}$ $\land$ $in\hbox{-}w(n,i)$}

\Indent
% \State $view_{\confirmation}$:= v
\State \hskip0.1em \mbox{$in_{\confirmation}:=in_{\confirmation}$ $\cup$ \{\preparej\}}
%\State $updatehash(in_{\confirmation})$
\EndIndent
\tikzmark{ff}
\EndIf
\EndProcedure

\end{algorithmic}
\end{algorithm}
\end{minipage}}

%\end{frame}

%%%%%%%%%%%%%%%%%%%%%%%%%%%%%%%%%%%%%%%%%

\newcommand\sendcommitm[3][]{%
  \begin{tikzpicture}[remember picture,overlay]
    \draw[overlay,fill=blue!30,#1] 
    ([xshift=-17em,yshift=-1ex]{pic cs:#2}) 
    rectangle 
    ([xshift=1cm,yshift=-1.5ex]pic cs:#3);
  \end{tikzpicture}%
}

%%%%%%%%%%%%%%%%%%%%%%%%%%%%%%%%%%%%%%%%%

%%%%%%%%%%%%%%%%%%%%%%%%%%%%%%%%%%%%%%%%%

%\begin{frame}{Send Commit}
 \scalebox{0.8}{
    \begin{minipage}{\linewidth}
\sendcommitm{gg}{hh}
\begin{algorithm}[H]
    \begin{algorithmic}[1]

\Procedure{\sendcommit$(m,v,n)_{\confirmation}$}{}
\tikzmark{gg}
\State Pre: $prepared(m,v,n,i)$  $\land$ \commiti $\notin$ $in_{\confirmation}$ 
\State Eff: let $c$= \commiti
\Indent
\State \hskip1em $view_{\confirmation}$ := v
\State \hskip1em $in_{\confirmation}:=in_{\confirmation}$ $\cup$ \{$c$\}
\State \hskip1em $in_{\confirmation}:=in_{\confirmation}$ $\cup$ \{\prepreparej, $p$\}
\tikzmark{hh}
\State \hskip1em $out_{\confirmation}:=out_{\confirmation}$ $\cup$ \{$c$\}
\EndIndent
\EndProcedure

\end{algorithmic}
\end{algorithm}
\end{minipage}
}

%\end{frame}

%%%%%%%%%%%%%%%%%%%%%%%%%%%%%%%%%%%%%%%%%
\newcommand\eone[3][]{%
  \begin{tikzpicture}[remember picture,overlay]
    \draw[overlay,fill=red!30,#1] 
    ([xshift=-14em,yshift=-1ex]{pic cs:#2}) 
    rectangle 
    ([xshift=5cm,yshift=0ex]pic cs:#3);
  \end{tikzpicture}%
}

\newcommand\etwo[3][]{%
  \begin{tikzpicture}[remember picture,overlay]
    \draw[overlay,fill=red!30,#1] 
    ([xshift=-5em,yshift=-14ex]{pic cs:#2}) 
    rectangle 
    ([xshift=9cm,yshift=17ex]pic cs:#3);
  \end{tikzpicture}%
}

%%%%%%%%%%%%%%%%%%%%%%%%%%%%%%%%%%%%%%%%%

%\begin{frame}{Execution}
  \scalebox{0.8}{
    \begin{minipage}{\linewidth}

 \eone{xa}{xd}
 \etwo{ya}{yd}
\begin{algorithm}[H]
   % \caption{Text Summarization Algorithm}\label{euclid}

    \begin{algorithmic}[1]

\newcommand{\lastexec}{$last\mbox{-}exec_{\execution}$ }
\newcommand{\lastrept}{$last\mbox{-}rep\mbox{-}t_{i}$(c) }
\newcommand{\lastrepi}{$last\mbox{-}rep_{i}$(c) }
\newcommand{\signDigest}{D($\langle$ val,\lastrepi,\lastrept$\rangle$) }
\newcommand{\checkpmessage}{$\langle$\checkp,$view_{\execution}$, $n$, \signDigest,$i$$\rangle \subrangle{\execution}$ }
\newcommand{\nestm}{$\langle$ $val_{i}$,\lastrept,\lastrepi $\rangle$ }
\newcommand{\cpmessage}{$\langle$ \textit{n},\nestm $\rangle \subrangle{\execution}$ }
\newpage

%% Execute
\Procedure{\execute$(m,v,n)_{\execution}$}{}
 \tikzmark{xa}
\State  Pre: n= \lastexec +1 $\land$ $committed(m,v,n)$ 
%// \textbf{the execution enclave needs to know the result of prepared predicate which is in the confirmation enclave}
\State Eff: \lastexec :=n
 \If {($m$ $\neq$ null)}
\If {$\exists$ $o$,$t$,$c$: (m=\clientreq)}
\If {$t$ $\geq$ \lastrept }
\If {$t$ $>$ \lastrept }
\State \lastrept := $t$ 
\State (\lastrepi, $val_{i}$):= g($c$,$o$,$val_{i}$)
 \tikzmark{xd}
\State  \mbox{$out_{i}:=out_{i}$ $\cup$ \{\replysig\}}

\EndIf
\EndIf
 \tikzmark{ya}
\State $in_{\execution}$ := $in_{\execution}$ - \{$m$\}
\If {$take\mbox{-}chkpt(n)$}
\State \mbox{let $m$$'$ = \checkpmessage}
\State $in_{\execution}$ := $in_{\execution}$ $\cup$ \{$m$$'$\} 
\State \mbox{$chkpts_{\execution}$ :=  $chkpts_{\execution}$ $\cup$ \{\cpmessage\}}
\State \out := \out $\cup$ \{$m$$'$\}
 \tikzmark{yd}
\EndIf
\EndIf
\EndIf

\EndProcedure

\end{algorithmic}
\end{algorithm}
\end{minipage}}
%\end{frame}
